# Supplementary material for: Causal Intervention for Fairness in Multi-behavior Recommendation
Source: arXiv:2209.04589 source file (2024-04-17)
Supplement: Supplementary file 1 [file 7_appendix.tex]

\section{Recommendation considering impact of popularity on click and post-click}\label{appendix}
In the previous sections, we only consider the impact of item popularity on post-click behavior. Moreover, we also take into account the situation that item popularity has an impact on both click and post-click behaviors. However, the derivation and our experiments show that 1) The causal intervention on item $I$ by adjusting popularity can remove the impact of the confounder popularity on click and post-click at the same time. The difference of considering the item popularity on click or not is to adjust item popularity on click and post-click separately or combined as one factor. 
% The intervention mechanism on item has not changed due to the consideration of popularity impact on click.
2) Considering the impact of item popularity on click behavior does not improve the recommendation effect, but also makes the model more redundant and complex. Therefore, this paper only considers the impact of popularity on post-click behavior.

The causal graph which considers the impact of item popularity on both click and post-click behavior is shown in Figure \ref{fig:both behavior}. In addition to the two backdoor paths $I \leftarrow Z \rightarrow L$ and $Z \leftarrow T \rightarrow Q \rightarrow L$, considering the impact of $Z \rightarrow C$, $Z$ is a confounder between item exposure and item click probability. To remove the backdoor path between $Z$ and $C$, we use the same causal intervention on $I$ to cutoff the backdoor path $I \leftarrow Z \rightarrow C$.

% We perform the intervention $do(I=i)$ by controlling the observed variable $Z$ to block the backdoor path $I \leftarrow Z \rightarrow L$ and achieve the intervention on $Q$ by controlling $Z$, which also blocks the second backdoor path.
The post-click probability $P(L|U, do(I), do(Q))$ is derived as the following Equation \eqref{equ:P_do_IQ_both_pop}:
\begin{subequations}
\label{equ:P_do_IQ_both_pop}
\begin{align}\footnotesize
&P(L|U,do(I),do(Q))=P_{G^\prime}(L| U,I,Q) \notag \\
                &=\sum_{Z_c}\sum_{Z_l}\sum_{C}{P_{G^\prime}(L| U,I,Q,Z_l,Z_c,C)P_{G^\prime}(C|U,I,Q)}P_{G^\prime}(Z_l| U,I,Q)P_{G^\prime}(Z_c| U,I,Q) \\
                &=\sum_{Z_c}\sum_{Z_l}\sum_{C}{P_{G^\prime}(L|U,I,Q,Z_l,Z_c,C)P_{G^\prime}(C|U,I)}P_{G^\prime}(Z_l)P_{G^\prime}(Z_c) \\
                &=\sum_{Z_c}\sum_{Z_l}P_{G^\prime}(L|U,I,Q,Z_l,Z_c,C=1)P_{G^\prime}(C=1|U,I)P_{G^\prime}(Z_l)P_{G^\prime}(Z_c)+ \\
                & \sum_{Z_c}\sum_{Z_l}P_{G^\prime}(L|U,I,Q,Z_l,Z_c,C=0)P_{G^\prime}(C=0|U,I)P_{G^\prime}(Z_l)P_{G^\prime}(Z_c) \notag \\
                &\approx\sum_{Z_c}\sum_{Z_l}P_{G^\prime}(L|U,I,Q,Z_l,C=1)P_{G^\prime}(C=1| U,I)P_{G^\prime}(Z_l)\\
                &=\sum_{Z_c}\sum_{Z_l}P(L|U,I,Q,Z_l,Z_c,C=1)P(C=1| U,I)P(Z_l)P(Z_c),
\end{align}
\end{subequations}
\begin{figure}[]
% \vspace{-2.5cm}
    \centering
    \includegraphics[width=.35\textwidth]{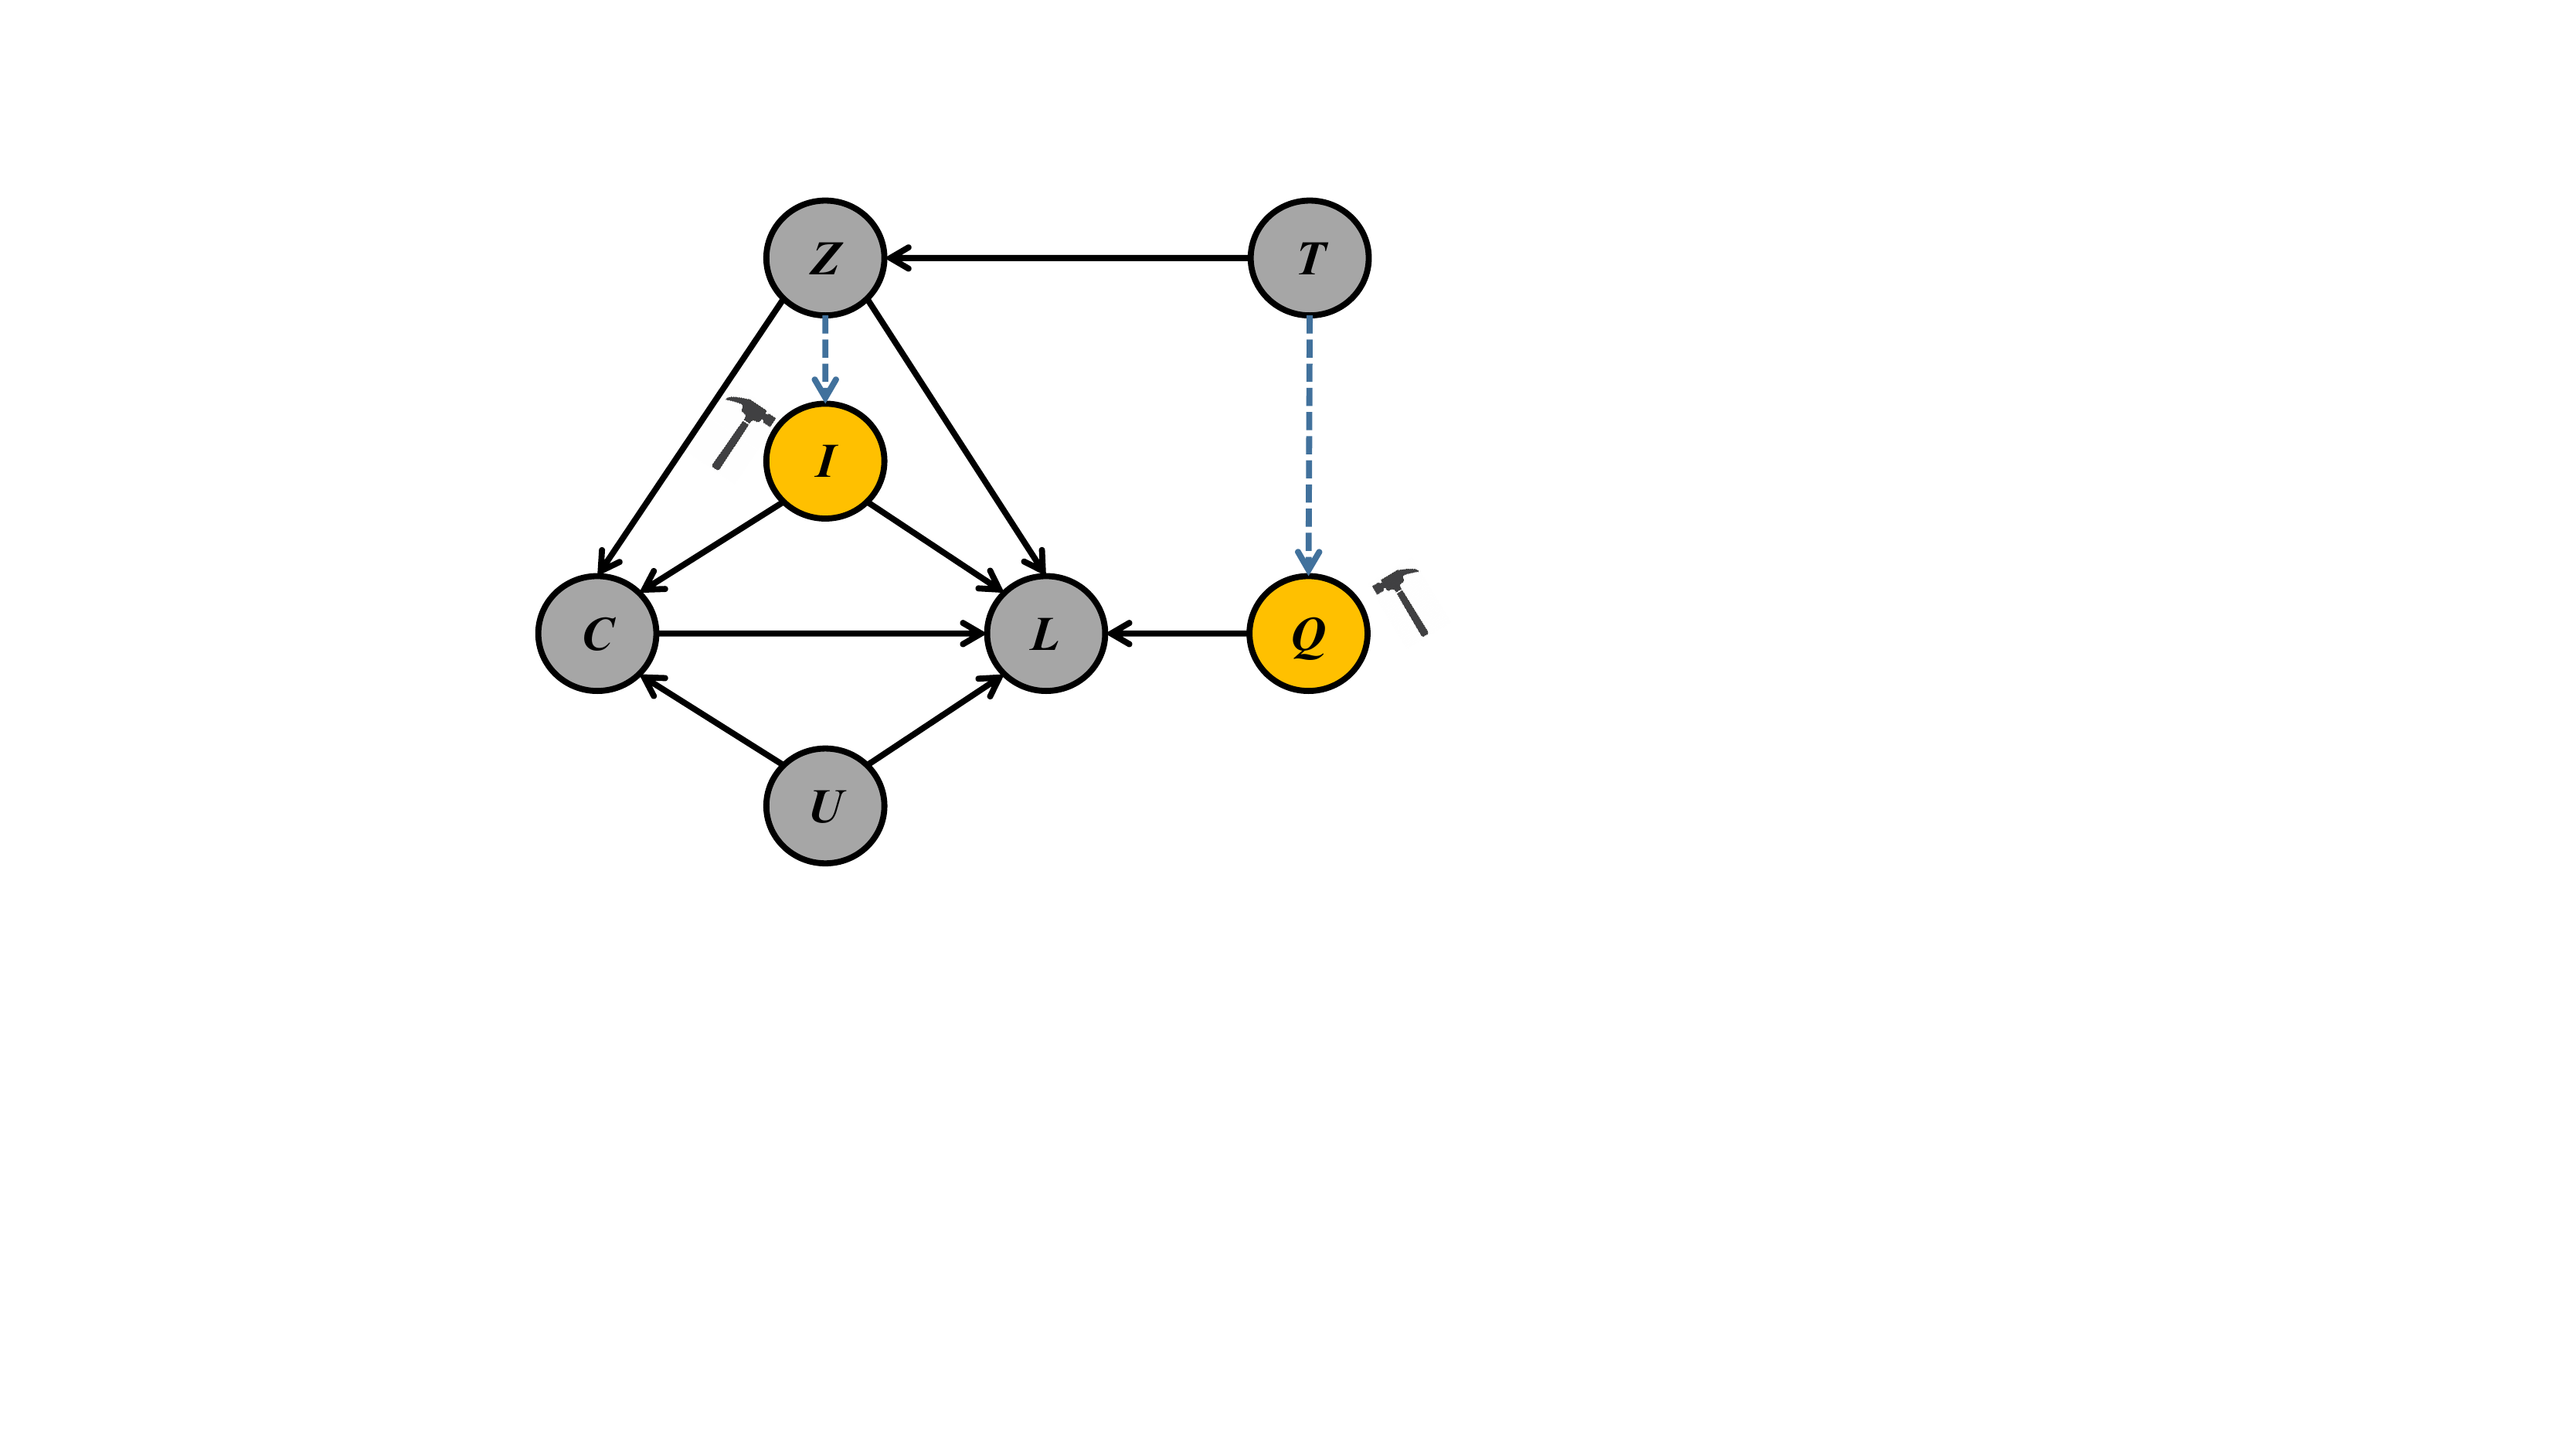} 
    \vspace{-5pt}
    \caption{Causal graph considering the impact of item popularity on click and post-click behaviors}
    \label{fig:both behavior}
    \vspace{-10pt}
\end{figure} 

As shown in the previous section \ref{sec:MBD_framework}, we can estimate the interventional probability $P(L|U,do(I),do(Q))$ as Equation \eqref{equ:both_pop} for simulation:

\begin{subequations}
\label{equ:both_pop}
\begin{align}\footnotesize
&P(L|U,do(I), do(Q)) \notag\\
                &=\sum_{Z_c}\sum_{Z_l}P(L|U,I,Q,Z_l,Z_c,C=1)P(C=1| U,I)P(Z_l)P(Z_c) \\
                &=\sum_{Z_c}\sum_{Z_l}\sigma(f_l(u,i))r_{i}^{\gamma_r} z_{i,l}^{\gamma_{z_l}}z_{i,c}^{\gamma_{z_c}}\sigma(f_{c}(u,i))p(Z_l)p(Z_c)   \\
                &=\sigma(f_{c}(u,i))\sigma(f_l(u,i))r_{i}^{\gamma_r}\sum_{Z_l} z_{i,l}^{\gamma_{z_l}}p(Z_l)\sum_{Z_c} z_{i,c}^{\gamma_{z_c}}p(Z_c)   \\
                &=\sigma(f_{c}(u,i))\sigma(f_l(u,i))r_{i}^{\gamma_r}E(Z^{\gamma_{z_l}})E(Z^{\gamma_{z_c}}),
\end{align}
\end{subequations}
where $E(Z^{\gamma_{z_c}})$ and $E(Z^{\gamma_{z_l}})$ are the expectations of $Z^{\gamma_{z_c}}$ and $Z^{\gamma_{z_l}}$ which are constants and do not change the recommendation results. Same as Figure \ref{fig:framework} shows, we use Equation~\eqref{equ:finalloss} to train the matching functions $f_{c}(u,i) $ and $f_l(u,i)$, and model the influence of the popularity $z_i$ and quality $r_i$ on $L$ at the training stage. Finally, we estimate the deconfounded prediction $s$ to rank item candidates as Equation \eqref{equ:score_inference}. Compared to the model only considering item popularity on post-click behavior, in the training, we add the expectation of the item popularity on click behavior and the hyper parameter $\gamma_{z_c}$. Because expectation depends on prior data, it increases the instability and complexity of the model.
